# Supplementary material for: Quantum Phase Transitions in Long-Range Interacting Hyperuniform Spin Chains in a Transverse Field
Source: arXiv:2012.06545 ancillary file (2020-12-14)
Supplement: Supplementary file 1 [file SM.pdf]

# Supplementary Material for Quantum Phase Transitions in Long-Range Hyperuniform Spin Chains in a Transverse Field

Amartya Bose

*Department of Chemistry, Princeton University, Princeton, New Jersey 08544*

Salvatore Torquato

*Department of Chemistry, Princeton University, Princeton, New Jersey 08544*

*Department of Physics, Princeton University, Princeton, New Jersey 08544*

*Princeton Institute for the Science and Technology of Materials,*

*Princeton University, Princeton, New Jersey 08544 and*

*Program in Applied and Computational Mathematics,*

*Princeton University, Princeton, New Jersey 08544*

## I. SIMULATION PARAMETERS

We considered Hamiltonians of the form:

$$H = -\sum_i \sum_{1 \le r \le R} J_r \hat{\sigma}_z^{(i)} \hat{\sigma}_z^{(i+r)} + \sum_i -\Gamma \hat{\sigma}_x^{(i)}. \tag{1}$$

in the paper. Here we list the three different parameters used in the section on hyperuniform spin chains:

| $r$ | $J_1(r)$ | $J_2(r)$ | $J_3(r)$ |
|---|---|---|---|
| 1 | 1 | 0.28571428571428555874 | 0.55769230769230704325 |
| 2 | 0.17754228440175393033 | -1 | 0.40624999999999961142 |
| 3 | 0.11776988932971439727 | -0.37662337662337647126 | 0.95673076923076916245 |
| 4 | 0.6767592399248280044 | 0.64610389610389584725 | 0.09374999999999472644 |
| 5 | 1 | 0.80735930735930749869 | 0.08173076923076835092 |
| 6 | 0.2787638337857594184 | -0.10064935064935048858 | 0.90144230769230759837 |
| 7 | 0.76894967634161570658 | -0.58441558441558449921 | 0.3173076923076922351 |
| 8 | 0.10471914804760995565 | 0.055194805194805192372 | 0.45673076923076860734 |
| 9 | 0.67675923992482822644 | 0.38961038961038968464 | 1 |
| 10 | 0.2388807684276468557 | 0.11147186147186152749 | |
| 11 | -0.332846105658801239 | -0.097402597402597379528 | |
| 12 | -0.24812069325537697284 | | |
| 13 | 0.37064105241177736083 | | |
| 14 | 1 | | |

In Sec. IIIB 1, we discussed the parameter with the single weak first-order phase transition. This corresponds to $J_1(r)$ and does not show a transition from disorder to order. In Sec. IIIB 2, we show results corresponding to $J_2(r)$, which shows one first-order transition and an increase in the $\tau$ order metric. Finally, $J_3(r)$ shows two first-order transitions (Sec. IIIB 3).
